# Supplementary material for: Chirality driven topological electronic structure of DNA-like materials
Source: arXiv:2008.08881 source file (2020-12-24)
Supplement: Supplementary file 1 [file SM.pdf]

# Supplementary Materials for "Chirality induced topological nature of electrons in DNA-like materials"

Yizhou Liu*, Jiewen Xiao*, Jahyun Koo, Binghai Yan†
Department of Condensed Matter Physics,Weizmann Institute of Science, Rehovot 76100, Israel
(Dated: December 24, 2020)

Section S1. Tight-binding model of the helical chain.
Section S2 and Figure S1. Anisotropic hopping along the chiral chain
Section S3 and Figure S2. Model parameters for the transport calculations.
Section S4 Scattering Matrix Method.
Figure S3. Band structures of the lead, the SOC region and the chiral molecule.
Figure S4. Band structures of the chiral molecule with a constant life time.
Figure S5. Band structure and transport calculations for broken $p_{x/y/z}$ degeneracy.
Figure S6. The total, orbital and spin conductance for chiral molecules with different length of units.
Figure S7. The comparison of the orbital filter effect and orbital polarization effect.
Figure S8. The comparison of the orbital filter effect and orbital polarization effect with different parameters.
Figure S9. Orbital channel-specific conductance of the chiral chain.
Figure S10. Verification of the global Onsager's reciprocal relation.
Figure S11. Influence of dephasing parameter $\eta$ on spin conductance.
Figure S12. Orbital channel-specific conductance of the achiral chain.
Figure S13. The orbital conserved lead and non-conserved lead in the achiral chain device.
Section S4 and Figure S14. The *ab intio* band structure of the chiral materials

## S1. TIGHT-BINDING MODEL

For the helix model with the three-fold skew rotation, there are three atomic sites $(R\cos(i-1)2\pi/3, R\sin(i-1)2\pi/3, z_0(i-1)(i=1,2,3)$ within the unit cell, where $i$ is the site number. We set the orbital bases $p_x, p_y, p_z$ on each site. The onsite energy of $p$ orbitals are set to zero while the nearest neighboring hopping is modelled by the Slater-Koster hopping. Therefore, the spinless Hamiltonian $H(k_z)$ can be expressed in the $p_{x,y,z}$ orbitals of three atomic sites,

$$H(k_z) = \begin{pmatrix} 0 & T_{12}exp(-ik_z \cdot a/3) & T_{13}exp(+ik_z \cdot a/3) \\ T_{21}exp(+ik_z \cdot a/3) & 0 & T_{23}exp(-ik_z \cdot a/3) \\ T_{31}exp(-ik_z \cdot a/3) & T_{32}exp(+ik_z \cdot a/3) & 0 \end{pmatrix}, \tag{S1}$$

where $1,2,3$ represent the atomic sites in the unitcell, $k_z$ and $a$ are the wave vector and lattice constant in the $z$ direction, respectively. $T_{ij}$ is the nearest-neighbor hopping matrix from site $i$ to site $j$ and can be written as

$$T_{ij}(\phi_{ij}, \theta_{ij}) = \begin{pmatrix} t_{ij,xx} & t_{ij,xy} & t_{ij,xz} \\ t_{ij,yx} & t_{ij,yy} & t_{ij,yz} \\ t_{ij,zx} & t_{ij,zy} & t_{ij,zz} \end{pmatrix} \tag{S2}$$

$$\begin{aligned} t_{ij,xx} &= t_\pi \sin^2\phi_{ij} + \cos^2\phi_{ij}(t_\sigma \sin^2\theta_{ij} + t_\pi \cos^2\theta_{ij}) \\ t_{ij,yy} &= t_\pi \cos^2\phi_{ij} + \sin^2\phi_{ij}(t_\sigma \sin^2\theta_{ij} + t_\pi \cos^2\theta_{ij}) \\ t_{ij,zz} &= t_\sigma \cos^2\theta_{ij} + t_\pi \sin^2\theta_{ij} \\ t_{ij,xy} &= t_{ij,yx} = \sin\phi_{ij}\cos\phi_{ij}(t_\sigma \sin^2\theta_{ij} - t_\pi \cos^2\theta_{ij}) \\ t_{ij,xz} &= t_{ij,xz} = \cos\phi_{ij}\sin\theta_{ij}\cos\theta_{ij}(t_\sigma - t_\pi) \\ t_{ij,yz} &= t_{ij,zy} = \sin\phi_{ij}\sin\theta_{ij}\cos\theta_{ij}(t_\sigma - t_\pi) \end{aligned} \tag{S3}$$

Here, $\phi_{ij}$ and $\theta_{ij}$ are the spherical coordinates of site $j$ relative to site $i$. For the helix molecule, $\theta_{ij}$ is set to $\pm\pi/4$ (so that $z_0 = 2\sqrt{3}R$), and $\phi_{ij}$ can adopt $\pm\pi/6, \pm 5\pi/6, \pm 3\pi/2$ value. For the hopping parameter, $t_\sigma$ and $t_\pi$ are 1.5 eV and -0.5 eV respectively. With the above parameter, band structure is calculated and shown in Figure 1(b).

## S2. ANISOTROPIC HOPPING ALONG THE CHIRAL CHAIN

In the last section, we derive the hopping matrix from site $i$ to site $j$ under $p_x, p_y, p_z$ bases. To understand the chiral selection from the anisotropic hopping, we write $T_{ij}$ under the $p_+, p_0, p_-$ orbital basis,

$$T_{ij}(\phi_{ij}, \theta_{ij}) = \begin{pmatrix} t_{ij,++} & t_{ij,+0} & t_{ij,+-} \\ t_{ij,0+} & t_{ij,00} & t_{ij,0-} \\ t_{ij,-+} & t_{ij,-0} & t_{ij,--} \end{pmatrix} \tag{S4}$$

$$\begin{aligned} t_{ij,++} &= (t_\pi(1+\cos^2\theta_{ij}) + t_\sigma \sin^2\theta_{ij})/2 \\ t_{ij,00} &= t_\sigma \cos^2\theta_{ij} + t_\pi \sin^2\theta_{ij} \\ t_{ij,--} &= (t_\pi(1+\cos^2\theta_{ij}) + t_\sigma \sin^2\theta_{ij})/2 \\ t_{ij,+0} &= t_{ij,0-} = ((t_\sigma - t_\pi)\sin\theta_{ij}\cos\theta_{ij}\exp(-i\phi_{ij}))/\sqrt{2} \\ t_{ij0,+} &= t_{ij,-0} = ((t_\sigma - t_\pi)\sin\theta_{ij}\cos\theta_{ij}\exp(+i\phi_{ij}))/\sqrt{2} \\ t_{ij,+-} &= ((t_\sigma - t_\pi)\sin^2\theta_{ij}\exp(-i2\phi_{ij}))/2 \\ t_{ij,-+} &= ((t_\sigma - t_\pi)\sin^2\theta_{ij}\exp(+i2\phi_{ij}))/2 \end{aligned} \tag{S5}$$

For the right-hand helical chain with the n-fold screw rotation, Figure S1 shows the electron hopping from site $i$ to adjacent site $i-1$ and site $i+1$, and such process can be denoted as 'd' (down) and 'u' (up) respectively. Therefore, the hopping matrix is written as $T_d = T_{i(i-1)}(\pi - \phi/2, -\theta)$ and $T_u = T_{i(i+1)}(\phi/2, \theta)$, and their relation can be further derived:

$$\begin{aligned} T_u &= \begin{pmatrix} t_{u++} & t_{u+0} & t_{u+-} \\ t_{u0+} & t_{u00} & t_{u0-} \\ t_{u-+} & t_{u-0} & t_{u--} \end{pmatrix} \\ &= \begin{pmatrix} t_{d++} \cdot e^{-i2\pi\cdot\Delta L_{z++}/n} & t_{d+0} \cdot e^{-i2\pi\cdot\Delta L_{z+0}/n} & t_{d+-} \cdot e^{-i2\pi\cdot\Delta L_{z+-}/n} \\ t_{d0+} \cdot e^{-i2\pi\cdot\Delta L_{z0+}/n} & t_{d00} \cdot e^{-i2\pi\cdot\Delta L_{z00}/n} & t_{d0-} \cdot e^{-i2\pi\cdot\Delta L_{z0-}/n} \\ t_{d-+} \cdot e^{-i2\pi\cdot\Delta L_{z-+}/n} & t_{d-0} \cdot e^{-i2\pi\cdot\Delta L_{z-0}/n} & t_{d--} \cdot e^{-i2\pi\cdot\Delta L_{z--}/n} \end{pmatrix} \end{aligned} \tag{S6}$$

Therefore, suppose there are two orbitals $p$ and $q$, the phase factor that connects the hopping term $t_{upq}$ and $t_{dpq}$ can be expressed as $e^{-i2\pi\cdot\Delta L_{zpq}/n}$, where $\Delta L_{zpq}$ is the z-component angular momentum ($L_z$) differences between orbital $p$ and orbital $q$. For the intra-orbital and inter-orbital hopping, we further have:

$$t_{u++} = t_{u--} = t_{d++} = t_{d--} \tag{S7}$$

$$t_{u00} = t_{d00} \tag{S8}$$

$$t_{u+-} = t_{d+-}e^{-i4\pi/n} \tag{S9}$$

$$t_{u+0} = t_{u0-} = t_{d+0}e^{-i2\pi/n} = t_{d0-}e^{-i2\pi/n} \tag{S10}$$

To validate the above $T_u$ and $T_d$ relation expressed by the differences of angular momentum, we further consider the $d$-orbital hopping in the chiral chain, with $L_z = 2, 1, 0, -1, -2$. Similarly, the hopping matrix from site $i$ to site $j$ under the $d_{2i}, d_{1i}, d_{0i}, d_{-1i}, d_{-2i}$ orbital basis can be written as:

$$T_{ij}(\phi_{ij}, \theta_{ij}) = \begin{pmatrix} t_{ij-2-2} & t_{ij-2-1} & t_{ij-20} & t_{ij-21} & t_{ij-22} \\ t_{ij-1-2} & t_{ij-1-1} & t_{ij-10} & t_{ij-11} & t_{ij-12} \\ t_{ij0-2} & t_{ij0-1} & t_{ij00} & t_{ij01} & t_{ij02} \\ t_{ij1-2} & t_{ij1-1} & t_{ij10} & t_{ij11} & t_{ij12} \\ t_{ij2-2} & t_{ij2-1} & t_{ij20} & t_{ij21} & t_{ij22} \end{pmatrix} \tag{S11}$$

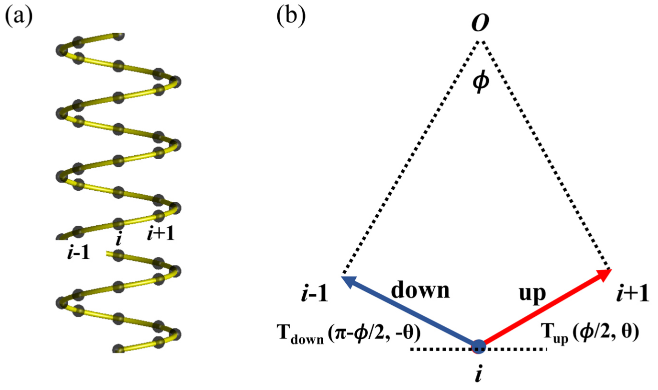


FIG. S1. Anisotropic hopping in the chiral chain. For the right hand helical chain, the hopping process from site $i$ to $i-1$ and from site $i$ to site $i+1$ can be denoted as 'd' (down) and 'u' (up), respectively.

$$\begin{aligned} t_{ij22} = t_{ij-2-2} &= (3t_\sigma - 4t_\pi + t_\delta)\sin^4\theta/8 + t_\pi \sin^2\theta + t_\delta \cos^2\theta \\ t_{ij11} = t_{ij-1-1} &= (3t_\sigma - 4t_\pi + t_\delta)\sin^2\theta\cos^2\theta/2 + t_\pi(1+\cos^2\theta) + t_\delta \sin^2\theta \\ t_{ij00} &= t_\sigma(\sin^2\theta - \cos^2\theta)^2/4 + 3t_\pi \sin^2\theta\cos^2\theta + 3t_\delta \sin^4\theta/4 \end{aligned} \tag{S12}$$

$$\begin{aligned} t_{ij21} = t^\dagger_{ij12} &= -t_{ij-1-2} = -t^\dagger_{ij-2-1} \\ &= (4(t_\delta - t_\pi)\sin 2\theta - (3t_\sigma - 4t_\pi + t_\delta)\sin^2\theta \sin 2\theta)e^{-i\phi} \\ t_{ij20} = t^\dagger_{ij02} &= t_{ij0-2} = t^\dagger_{ij-20} \\ &= (\sqrt{6}\sin^2\theta/8)(t_\sigma(\cos^2\theta - \sin^2\theta) - 4t_\pi\cos^2\theta + t_\delta(1+\cos^2\theta))e^{-i2\phi} \\ t_{ij2-1} = t^\dagger_{ij-12} &= -t_{ij1-2} = -t^\dagger_{ij-21} \\ &= (\sin 2\theta \sin^2\theta/8)(3t_\sigma - 4t_\pi + t_\delta)e^{-i3\phi} \\ t_{ij2-2} &= t^\dagger_{ij-22} \\ &= (\sin^4\theta/8)(3t_\sigma - 4t_\pi + t_\delta)e^{-i4\phi} \\ t_{ij10} = t^\dagger_{ij01} &= -t_{ij0-1} = -t^\dagger_{ij-10} \\ &= (\sqrt(3)\sin\theta\cos\theta/4)(t_\sigma(2\cos^2\theta - \sin^2\theta) - 2t_\pi\cos 2\theta + t_\delta \sin^2\theta)e^{-i\phi} \\ t_{ij1-1} &= t^\dagger_{ij-11} \\ &= (\sin^2\theta/2)((t_\delta - t_\pi) - (3t_\sigma - 4t_\pi + t_\delta)\cos^2\theta)e^{-i2\phi} \end{aligned} \tag{S13}$$

With $T_d = T_{i(i-1)}(\pi - \phi/2, -\theta)$ and $T_u = T_{i(i+1)}(\phi/2, \theta)$, the general relation between the matrix element $t_{upq}$ in $T_u$ and $t_{dpq}$ in $T_d$ can be written as (where $p$ and $q$ are $d$ orbitals, and $\Delta L_{zpq}$ is the $L_z$ difference between them):

$$t_{upq} = t_{dpq} exp(-i2\pi \cdot \Delta L_{zpq}/n) \tag{S14}$$

## S3. SCATTERING MATRIX METHOD

The scattering matrix $S_{nm}$ used in Eq. (1) of the main text is defined as the complex transmission amplitude from the $n$-th input state in the left lead $L$ to the $m$-th output state in the right lead $R$. The total conductance from $L$ to $R$ is

$$G_{L\to R} = \frac{e^2}{h}\sum_{n,m}|S_{nm}|^2 = \frac{e^2}{h}\mathrm{Tr}(S^\dagger S). \tag{S15}$$

Each matrix element of $S$ can be calculated through mode-matching method based on a tight-binding model [see T. Ando, Phys. Rev. B **44**, 8017 (1991) or P. A. Khomyakov, G. Brocks, V. Karpan, M. Zwierzycki, and P. J. Kelly, Phys. Rev. B **72**, 035450 (2005)].

Since the detailed formulation has been derived in different but equivalent forms and has been applied to different physical systems including phonons, we use the version of Chen et al. Phys. Rev. B **99**, 064302 (2019) and only give the final expression here without deriving it:

$$S_{nm} = \sqrt{\frac{v_{Rm}/a_R}{v_{Ln}/a_L}} \langle \bar{u}_{Rm}|G_{RL}(G_L^{\text{bulk}})^{-1}|u_{Ln}\rangle. \tag{S16}$$

$v_{Rm}$ ($v_{Ln}$) is velocity of $m$-th ($n$-th) state in the lead $R$ ($L$); $a_R$ ($a_L$) is the lattice constant; $G_{RL}$ is the solution of the following equation:

$$\left[E - \begin{pmatrix} H_L & V_{LC} & 0 \\ V_{CL} & H_C & V_{CR} \\ 0 & V_{RC} & H_R \end{pmatrix}\right]^{-1} = \begin{pmatrix} \cdots & \cdots & \cdots \\ \cdots & \cdots & \cdots \\ G_{RL} & \cdots & \cdots \end{pmatrix} \tag{S17}$$

where $E$ is the energy of incident electron, $H_{L(R)}$ is the Hamiltonian of a unit cell of lead $L$ ($R$), and $V_{LC} = V_{CL}^\dagger$ and $V_{CR} = V_{RC}^\dagger$ is the coupling between central region and leads; $G_L^{\text{bulk}}$ is the bulk Green function which can be numerically solved through a fast convergent scheme [see Sancho, M. P. L., Sancho, J. M. L., Sancho, J. M. L. & Rubio, J. "Highly convergent schemes for the calculation of bulk and surface Green functions," J. Phys. F **15**, 851–858 (1985)]; $|u_{Ln}\rangle$ is the wave function of $n$-th state of lead $L$ at given energy $E$ with positive velocity (which means velocity pointing from lead $L$ to $R$) which are solved by the generalized eigenvalue equation: $A_L|\psi_{Ln}\rangle = \lambda_{Ln}B_L|\psi_{Ln}\rangle$ with $|\lambda_{Ln}| = 1$ where

$$A_L = \begin{pmatrix} V_L^\dagger & H_L \\ 0 & \mathbb{I}_L \end{pmatrix}, \qquad B_L = \begin{pmatrix} E & -V_L \\ \mathbb{I}_L & 0 \end{pmatrix}, \qquad |\psi_{Ln}\rangle = \begin{pmatrix} |u_{Ln}\rangle \\ \lambda_{Ln}|u_{Ln}\rangle \end{pmatrix}, \tag{S18}$$

where $V_L$ is the coupling between adjacent unit cells; $\langle \bar{u}_{Rm}|$ is determined by $\langle \bar{u}_{Rm}|u_{Rm'}\rangle = \delta_{mm'}$. Since matrix $A$ and $B$ are not Hermitian, $\langle \bar{u}_{Rm}|$ does not equal to the Hermitian conjugate of $|u_{Rm}\rangle$.

For $G_L$ and $G_S$, the angular momentum conductance $G_J$ ($J = L, S$ for orbital and spin, respectively) is defined as

$$G_J = \frac{e^2}{h}\text{Tr}(S^\dagger J S) \tag{S19}$$

where $J$ is the angular momentum matrix in the basis of output lead eigenstates. For $J$-conserved output lead the $J$ matrix is diagonal: $J_{m'm} = j_m \delta_{m'm}$, where $j_m$ is the eigenvalue of $J$ and $\delta_{m'm}$ is the Kronecker function [i.e. $\delta_{m'm} = 1$ (0) for $m' = m$ ($m' \neq m$)]. The expression of $G_J$ reduces to

$$G_J = \frac{e^2}{h}\sum_{n,m} j_m |S_{nm}|^2, \tag{S20}$$

where $j_m = +1, 0, -1$ for orbital conductance, and $j_m = \pm 1/2$ for spin conductance. Equation (S17) has the physical meaning of how many (orbital or spin) angular momentum the transmitted current carries.

## S4. MODEL PARAMETERS AND BAND STRUCTURES

Hopping parameters for the two terminal device are presented in Figure S2, and their values are specified in the attached codes. To calculate the orbital channel-specific conductance of the achiral chain, we set the isotropic hopping $t$ in leads. We also test the spin channel-specific conductance for both the isotropic hopping ($t = t_\sigma = t_\pi = 1.3$ eV, orbital $L_x$ conserved) and the general anisotropic hopping ($t_\sigma = 1.5$ eV, $t_\pi = 1.3$ eV, orbital $L_x$ non-conserved) in leads, and results in Figure S6 display the similar feature.

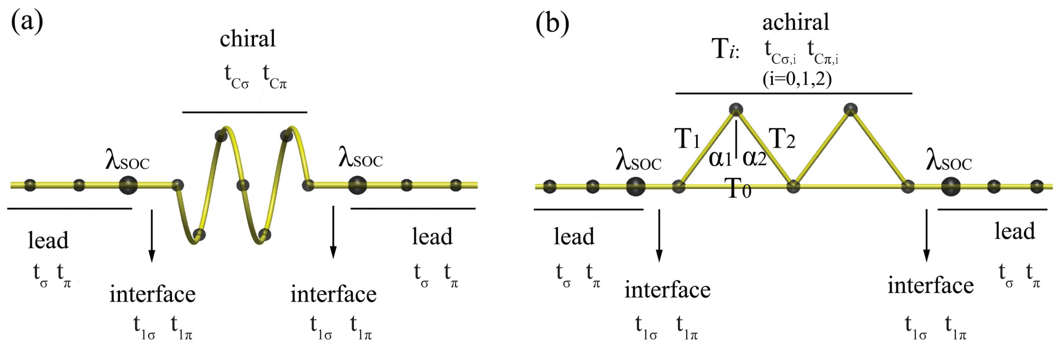


FIG. S2. Hopping parameters for the two-terminal device: (a) chiral molecule, and (b) achiral molecule.

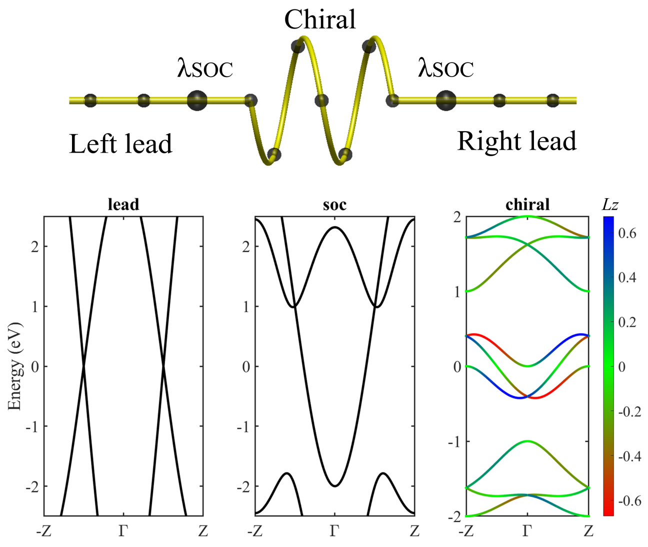


FIG. S3. Band structures of the lead, the SOC region and the chiral molecule. The chiral molecule is represented by the right-hand helix model discussed above and related hopping parameters and SOC strength are detailed in the section S4.

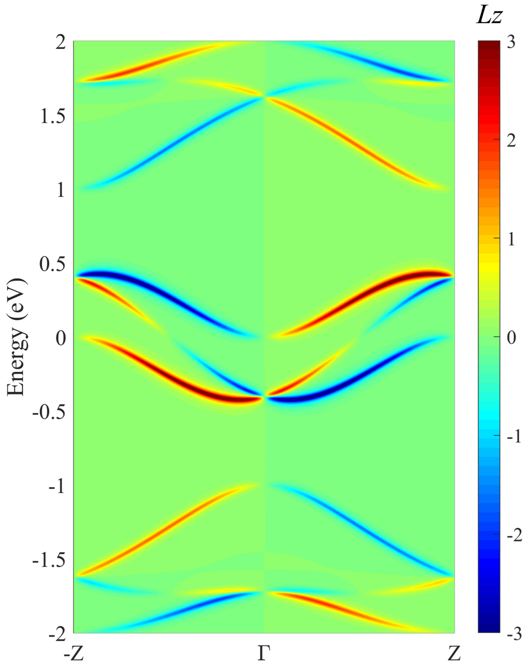


FIG. S4. Band structures of the chiral molecule with a constant life time $\tau$. The lifetime effect of quasiparticles is considered by setting a finite dephasing term $\eta = \hbar/\tau = 0.02$ eV. The orbtial angular momentum $L_z$ can still be projected into the band structure, which demonstrates the robust orbital texture under the many body effects. We used the same parameters as those for Fig.1b

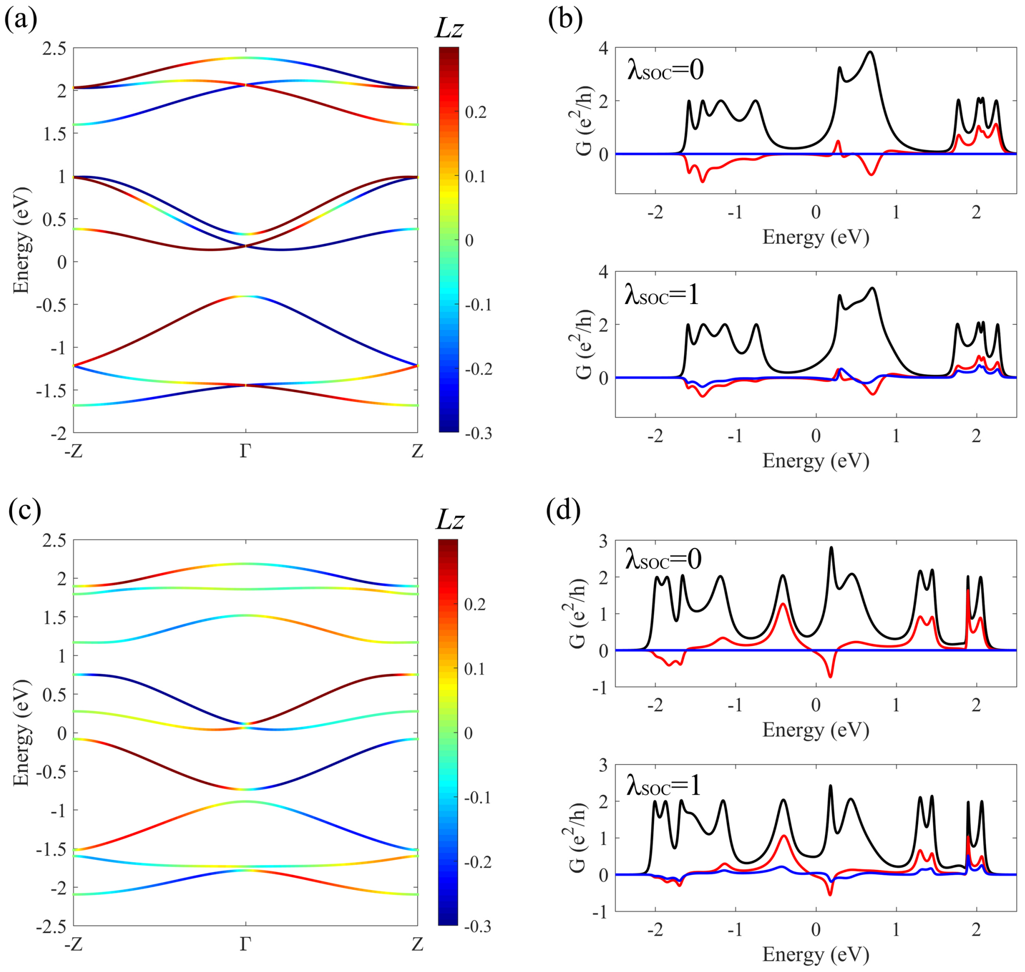


FIG. S5. The band structure ((a) and (b)) and transport calculations ((c) and (d)) for chiral molecules with the broken $p_{x/y/z}$ degeneracy. For (a) and (b), we set onsite energies of $p$ orbitals as $\Delta_{p_x} = \Delta_{p_y} = 0.6$ eV and $\Delta_{p_z} = 0.1$ eV, which breaks the $p_z$ and $p_{x/y}$ degeneracy and preserves the chiral symmetry. For (c) and (d), we set onsite energies as $\Delta_{p_x} = 0.6$ eV, $\Delta_{p_y} = -0.4$ eV and $\Delta_{p_z} = 0.0$ eV, which even breaks the chiral symmetry. The other parameters are the same as Fig.1b and Fig.2. In both cases, the orbital texture and further the induced orbital and spin conductance are always preserved. It is worth to note that, we have band gaps in both cases, but such band gap opening does not affect our results.

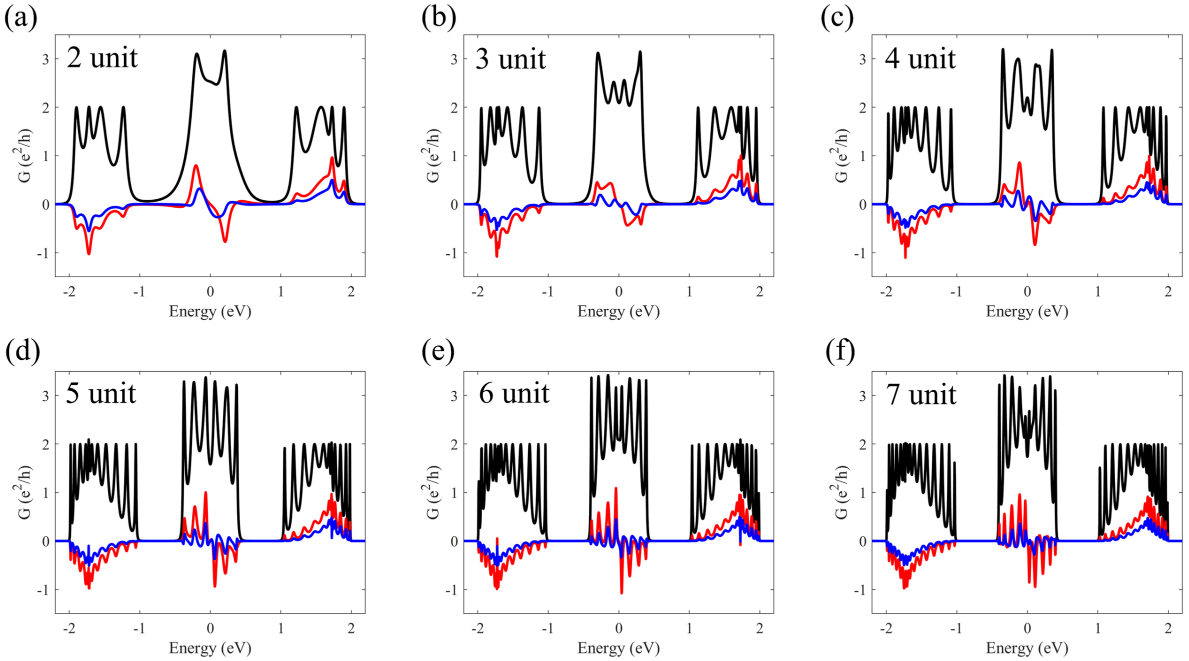


FIG. S6. The total, orbital and spin conductance for chiral molecules with different length of units. With the increasing molecular length, the tunneling effect is gradually weakened and the conductance turns to be zero in the band gap. The other parameters and device configuration are the same as those in Fig. 2.

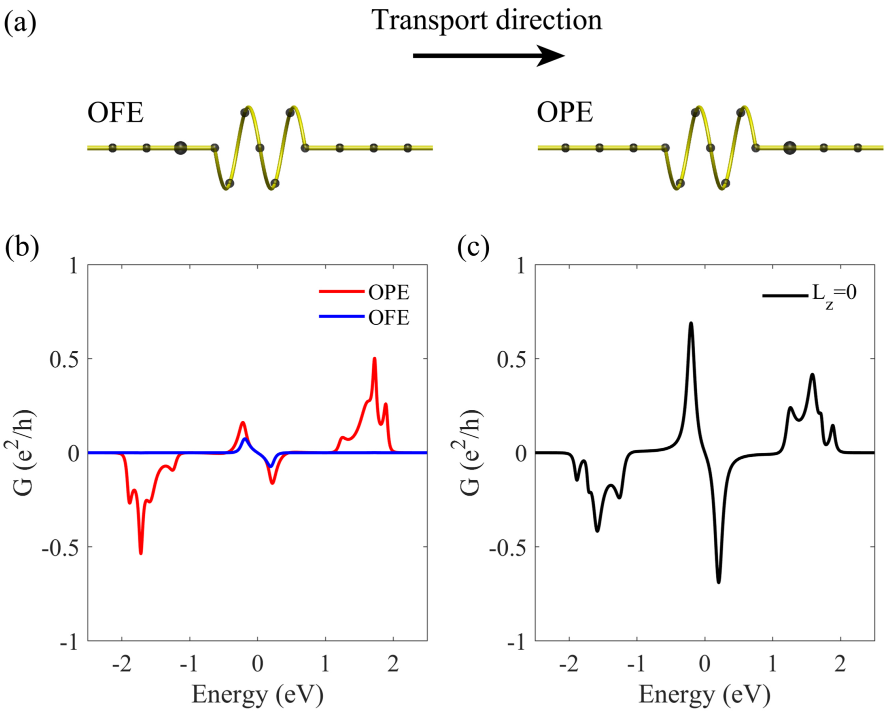


FIG. S7. The comparison of the orbital filter effect (OFE) and orbital polarization effect (OPE). (a) Schematic representation of OFE and OPE, where the SOC region is placed before and after the chiral molecule. (b) Spin conductance for the OFE and OPE device, where OPE is much more effective than OFE. (c) The orbital conductance for the initial injected $L_z = 0$ orbital, where the positive/negative conductance means $L_0$ state is converted into $L_\pm$ state (SOC strength is set to zero). Under the orbital texture of the chiral molecule, the initial $L_z = 0$ orbital will be polarized and transformed into spin current in the OPE device. This scenario can be further verified by the similar distribution pattern of the $L_z = 0$ orbital conductance and spin conductance in OPE.

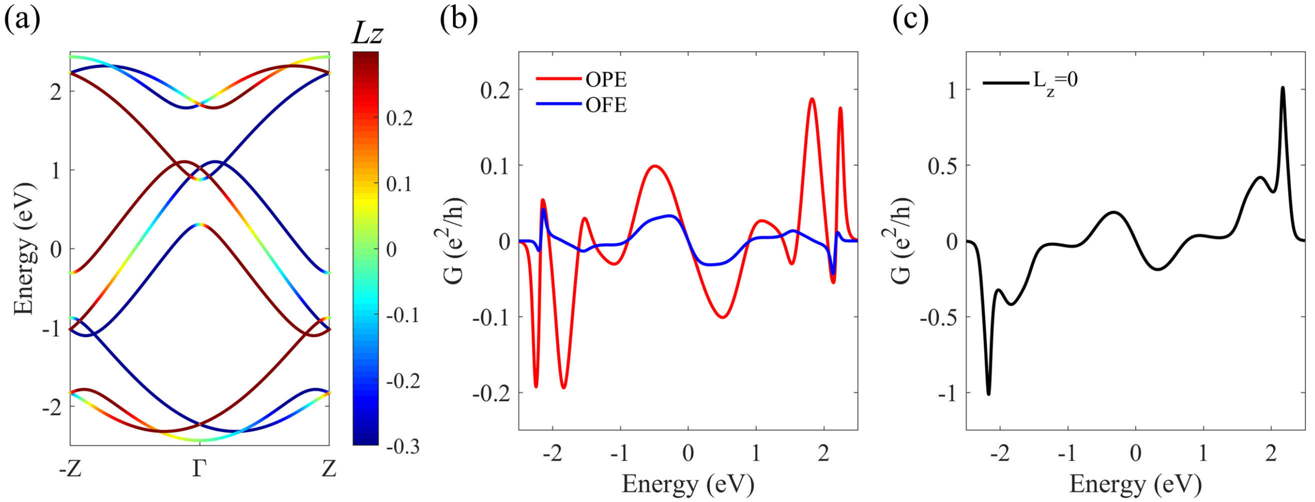


FIG. S8. The comparison of the orbital filter effect (OFE) and orbital polarization effect (OPE) with different parameters. (a) Band structure of the chiral molecule with another set of hopping parameters as: $t_\sigma = -1.5$ eV and $t_\pi = 1.0$ eV in the chiral region. (b) The spin conductance for the OFE and OPE device, where OPE is still more effective than OFE. (c) The orbital conductance for the initial injected $L_z = 0$ orbital (SOC strength is set to zero). The orbital conductance pattern is still similar to the enhanced spin conductance in OPE, further demonstrating the orbital-spin conversion scenario in OPE.

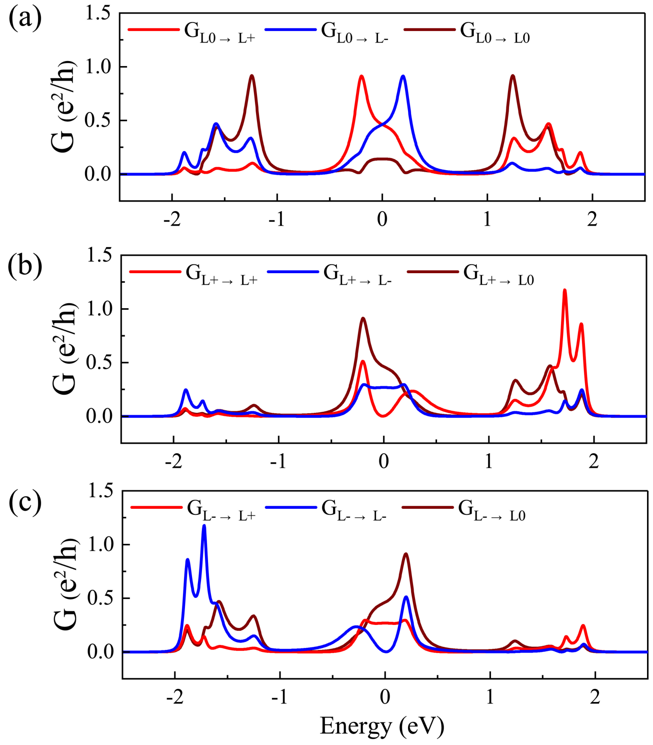


FIG. S9. Orbital channel-specific conductance of the chiral chain. Specific conductance from $L_+$, $L_0$, $L_-$ orbital channel in the left lead to the $L_+$, $L_0$, $L_-$ orbital channel in the right is presented (SOC strength is set to zero)

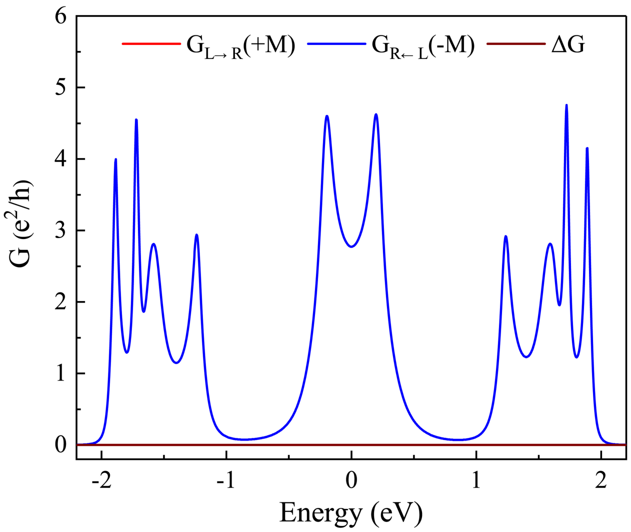


FIG. S10. Verification of the global Onsager's reciprocal relation. When dephasing term $\eta$ is set to zero, $\Delta G = G_{L\to R}(M) - G_{R\to L}(-M) = 0$.

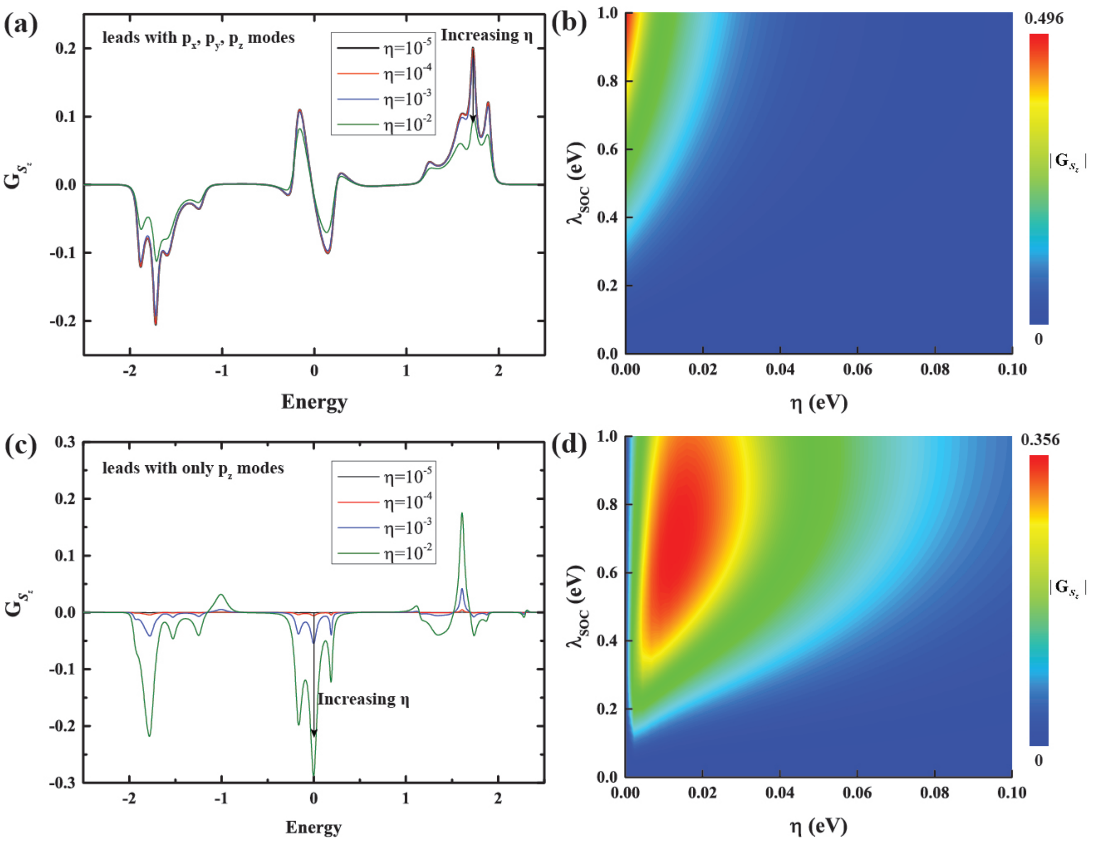


FIG. S11. Influence of dephasing parameter $\eta$ on spin conductance $G_{S_z}$ of (a)-(b) multiple-mode leads and (c)-(d) single-mode leads, respectively. (a), (c) $G_{S_z}$ as function of energy for various $\eta$. (b), (d) $G_{S_z}$ as function of $\eta$ and $\lambda_{\rm SOC}$ at fixed energy (indicated by the arrows in (a) and (c), respectively). The single-mode leads are created by setting $t_\pi^{\rm leads} = 0$ so that only $p_z$ modes (with two spins) contribute to spin and charge transport. For single-mode leads a finite dephasing is needed to generate nonzero $G_{S_z}$ whereas for multiple-mode leads it is not necessary.

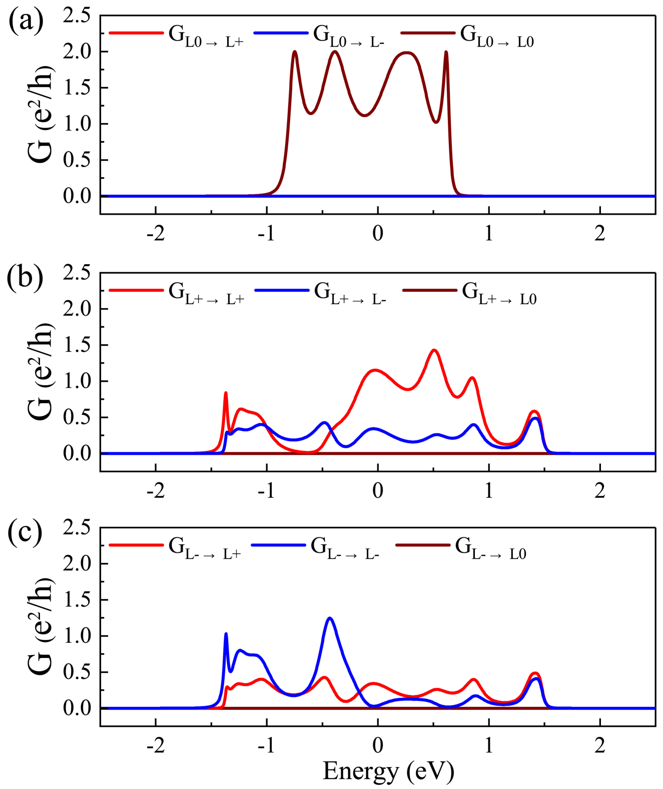


FIG. S12. Orbital channel-specific conductance for the achiral chain. Nine kinds of conductance from $L_+$,$L_0$,$L_-$ orbital channel in the left lead to the $L_+$,$L_0$,$L_-$ orbital channel in the right lead are presented (SOC strength is set to zero.)

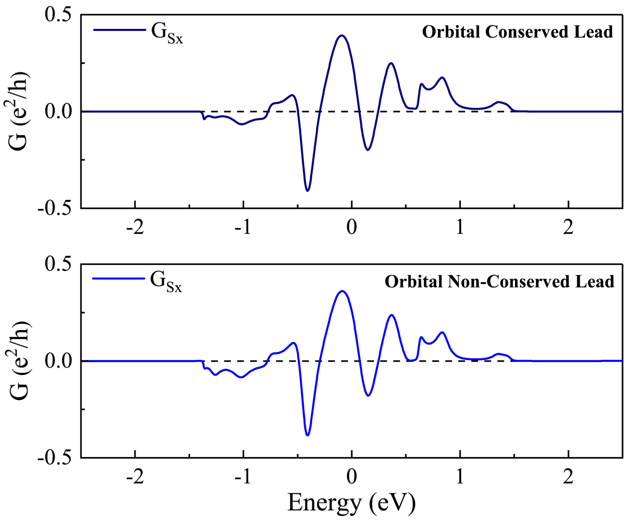


FIG. S13. Spin conductance $G_{Sx}$ for the $L_x$ orbital conserved lead and non-conserved lead in the achiral chain device. Detailed hopping parameters are shown in section S4.

## S5. THE *AB INTIO* BAND STRUCTURE OF THE CHIRAL MATERIALS

We calculate a $3_{10}$ helix and $\alpha$-helix structure to show the robust orbital texture of the chiral materials. We employ the $3_{10}$ helix and the $\alpha$-helix structure as poly-alaline($C_3H_7NO_2$) peptide. There are 3(3.6) residues/turn in the $3_{10}$ helix($\alpha$-helix). To make the molecule as a crystal structure we use 3 residues for the $3_{10}$ helix and 18 residues for the $\alpha$ helix. For the $3_{10}$ helix there is one residue every 120 degree follows the three-fold screw rotation (spiral symmetry). For the $\alpha$ helix, three residues in every 300 degree, thus three residues together follows the six-fold screw rotation. Each residue is translated 2 Åand 1.5 Å along the vertical direction for the $3_{10}$ and $\alpha$ helix, respectively. The band degeneracy at the $\Gamma$ and $\pm Z$ points are caused by the screw rotational symmetry. The calculated band gap of the $3_{10}$ and $\alpha$ helix is 4.6 eV (Figure 1 (a) in the main text) and 4.3 eV(Figure S14 (a)), respectively.

Even with breaking the spiral symmetry, the orbital texture preserves. For example, we calculated the band structure of the $3_{10}$ helix with reduced symmetry (Figure S14 (b)). We changed one of the functional group(side-chain) in the chiral structure to different one(from -$CH_3$(alanine) to -$CH_2C_5H_6$(phenylalanine)). The orbital texture still remains, although the band degeneracy is lifted off for the $\Gamma$ and $\pm Z$ points.

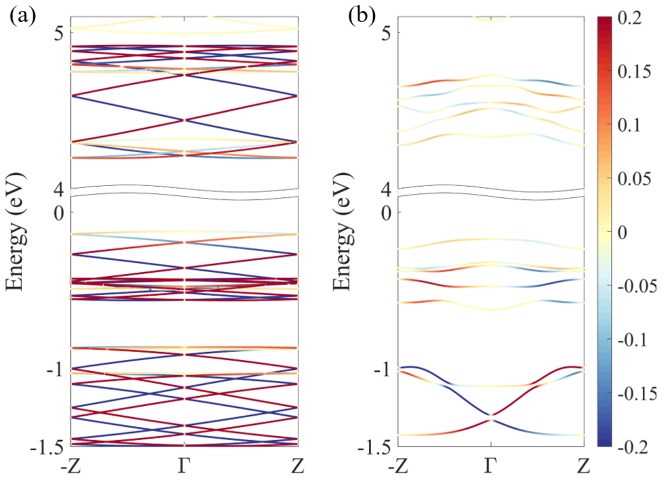


FIG. S14. The *ab-intio* calculation result. (a) The calculated band structure with orbital momentum of the right-handed $\alpha$-helix with orbital texture. (b) The calculated band structure with orbital momentum of $3_{10}$ helix with the spiral symmetry-breaking.
